# Supplementary material for: Transition Matrix Representation of Trees with Transposed Convolutions
Source: arXiv:2202.10677 source file (2022-02-22)
Supplement: Supplementary file 1 [file 100appendix.tex]

\section{Interpretability}

\subsection{Interpretability Measure}

Interpretability is the main advantage of tree models, but it is often ambiguous and hard to be measured.
For instance, a decision tree is commonly believed to be interpretable, but it is unclear whether the variants of decision trees such as soft decision trees \cite{Irsoy12} or deep neural decision trees \cite{Yang18a} with more complex decision functions are still interpretable, since there is no clear way to quantify the in interpretability of individual tree models.

\begin{figure}
        \centering
        \begin{subfigure}{0.24\textwidth}
                \includegraphics[width=\textwidth]{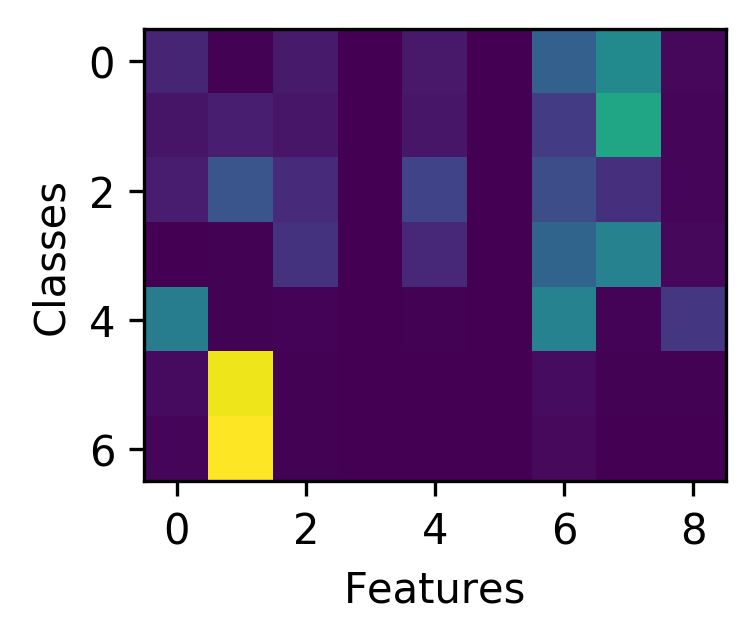}
                \caption{Logistic regression.}
%                \label{fig:structure-1}
        \end{subfigure} \hfill
        \begin{subfigure}{0.24\textwidth}
                \includegraphics[width=\textwidth]{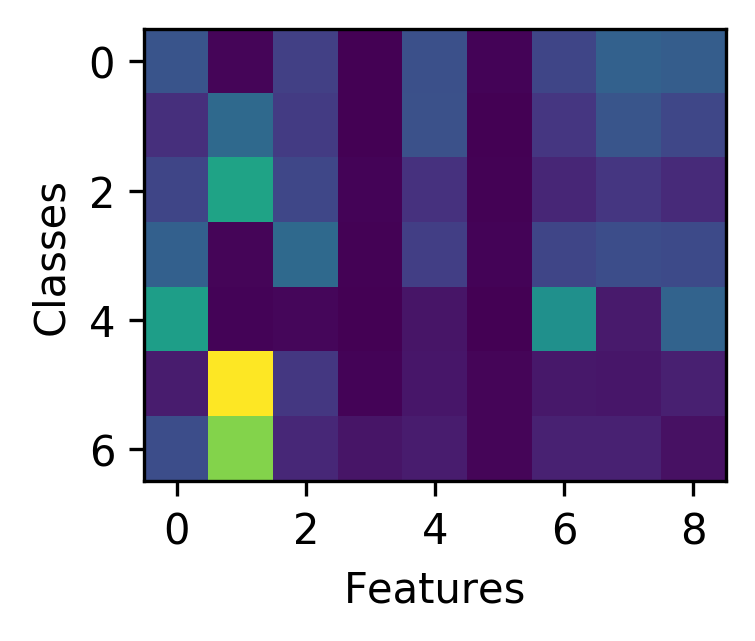}
                \caption{{\method}-A.}
%                \label{fig:structure-1}
        \end{subfigure}
        \caption{%
                Comparison of feature relevances in the \texttt{car} dataset for (a) logistic regression and (b) {\method}-A, summarized for all examples of each class.
%                Brighter colors represent larger values of relevance.
                They show similar patterns, indicating the features that are relevant to each target class.
        }
\label{fig:class-relevances}
\end{figure}

We show the interpretability of \method in terms of feature relevance, providing a way to measure the interpretability of any tree models based on the generalizability of our \method.
We start by presenting Definitions \ref{def:relevance} and \ref{def:interpretability} and make a statement about the interpretability of our \method in Theorem \ref{theorem:interpretability}.
%Thus, we provide a general way to measure the interpretability of tree models based on feature relevance scores. Relevance scores are used as a measure of interpretability for deep neural networks \cite{Montavon18}.

\begin{definition}
	Given a function $f$, let $v = f(\mathbf{x})$.
	Then, $r_k(v)$ is a relevance score for $x_k$ if $r_k(v)$ measures how relevant $x_k$ is for explaining $v$, and $\sum_k r_k(v) = v$.
\label{def:relevance}
\end{definition}

\begin{definition}
	A function $f$ is interpretable if $r_k(f(\mathbf{x}))$ exists for every $k$.
	A value $v$ is interpretable if it is a constant or generated from an interpretable function.
\label{def:interpretability}
\end{definition}

In other words, we define the interpretability of a function $f$ based on the existence of relevance scores.
It is known that in a special case of functions such as piecewise linear functions that satisfy $f(t\mathbf{x}) = tf(\mathbf{x})$ for $t \geq 0$, the relevance score is written as follows \cite{Montavon18}:
\begin{equation}
	r_k(f(\mathbf{x})) = \frac{\partial f(\mathbf{x})}{\partial x_k} x_k.
\label{eq:simplified-relevance}
\end{equation}

This applies also to our \method, which consists of linear transformations by transition matrices.
Based on Equation \eqref{eq:simplified-relevance}, we show as Lemmas \ref{prop:addition} and \ref{prop:multiplication} that the addition and multiplication of interpretable terms $v_1$ and $v_2$ are also interpretable, and the relevance scores are derived by simple propagation rules.
Then, we present Theorem \ref{theorem:interpretability} for the interpretability of \method in relation to the transition functions.

\begin{figure}
        \centering
        \begin{subfigure}{0.24\textwidth}
                \includegraphics[width=\textwidth]{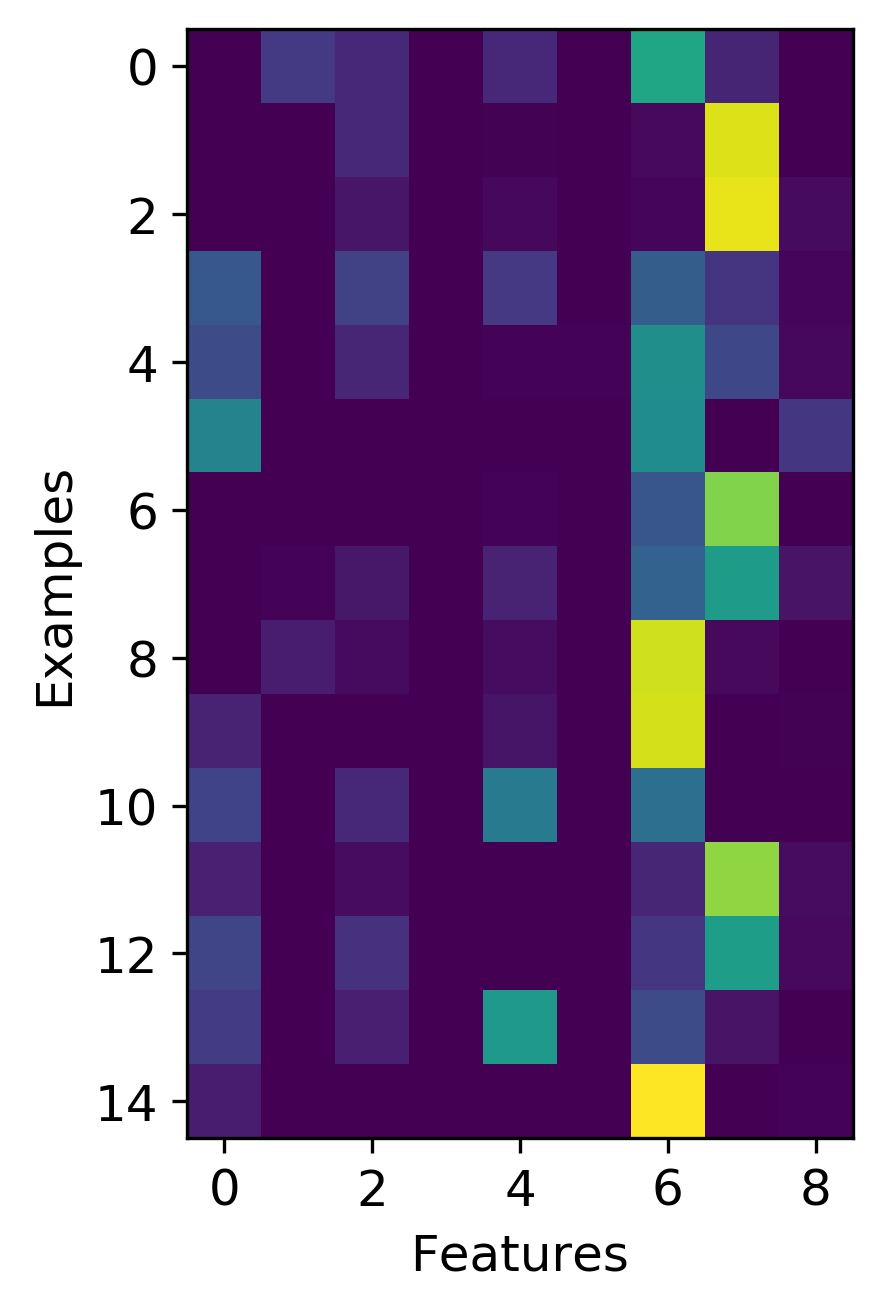}
                \caption{Logistic regression.}
%                \label{fig:structure-1}
        \end{subfigure} \hfill
        \begin{subfigure}{0.24\textwidth}
                \includegraphics[width=\textwidth]{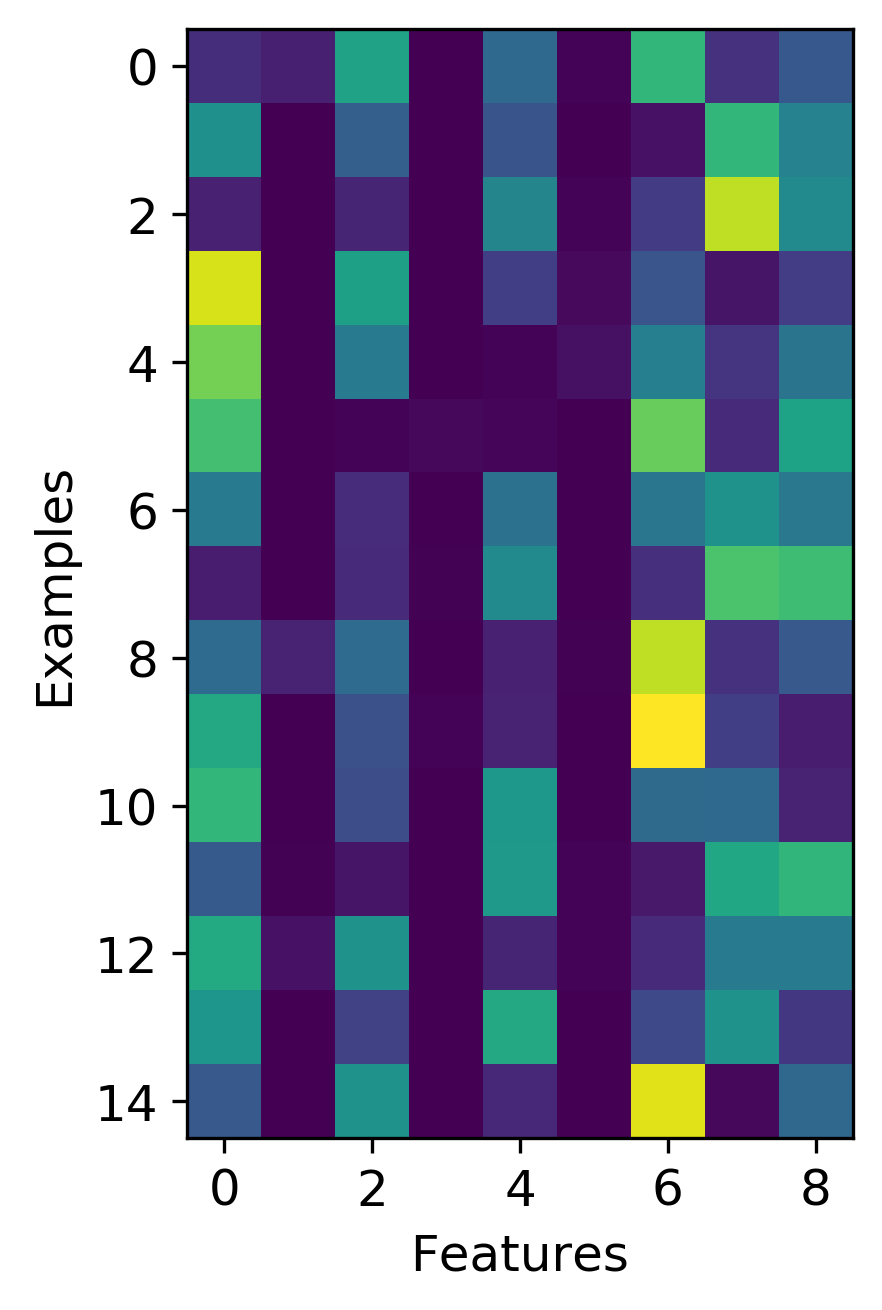}
                \caption{{\method}-A.}
%                \label{fig:structure-1}
        \end{subfigure}
        \caption{%
                Comparison of feature relevances in the \texttt{car} dataset, generated for (a) logistic regression and (b) {\method}-A.
                Brighter colors represent larger values of relevance.
                The scores follow similar patterns even with different classifiers.
        }
\label{fig:relevances}
\end{figure}

\begin{figure*}
        \centering
        \begin{subfigure}{0.32\textwidth}
                \includegraphics[width=\textwidth]{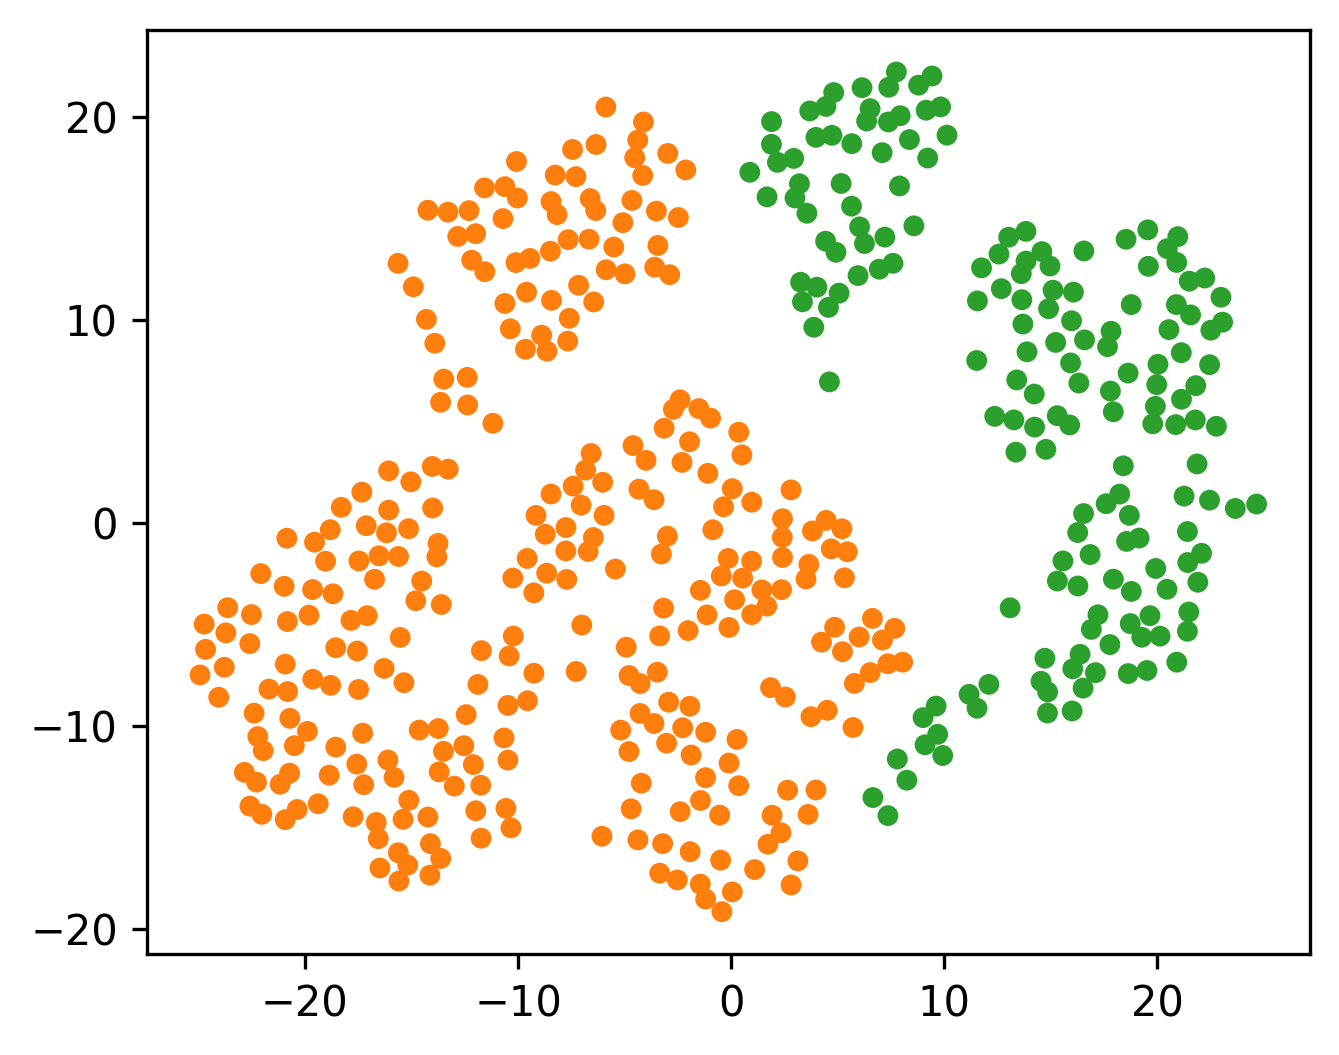}
                \caption{Arrived nodes at layer 1.}
                \label{fig:prototypes-1}
        \end{subfigure}
        \begin{subfigure}{0.32\textwidth}
                \includegraphics[width=\textwidth]{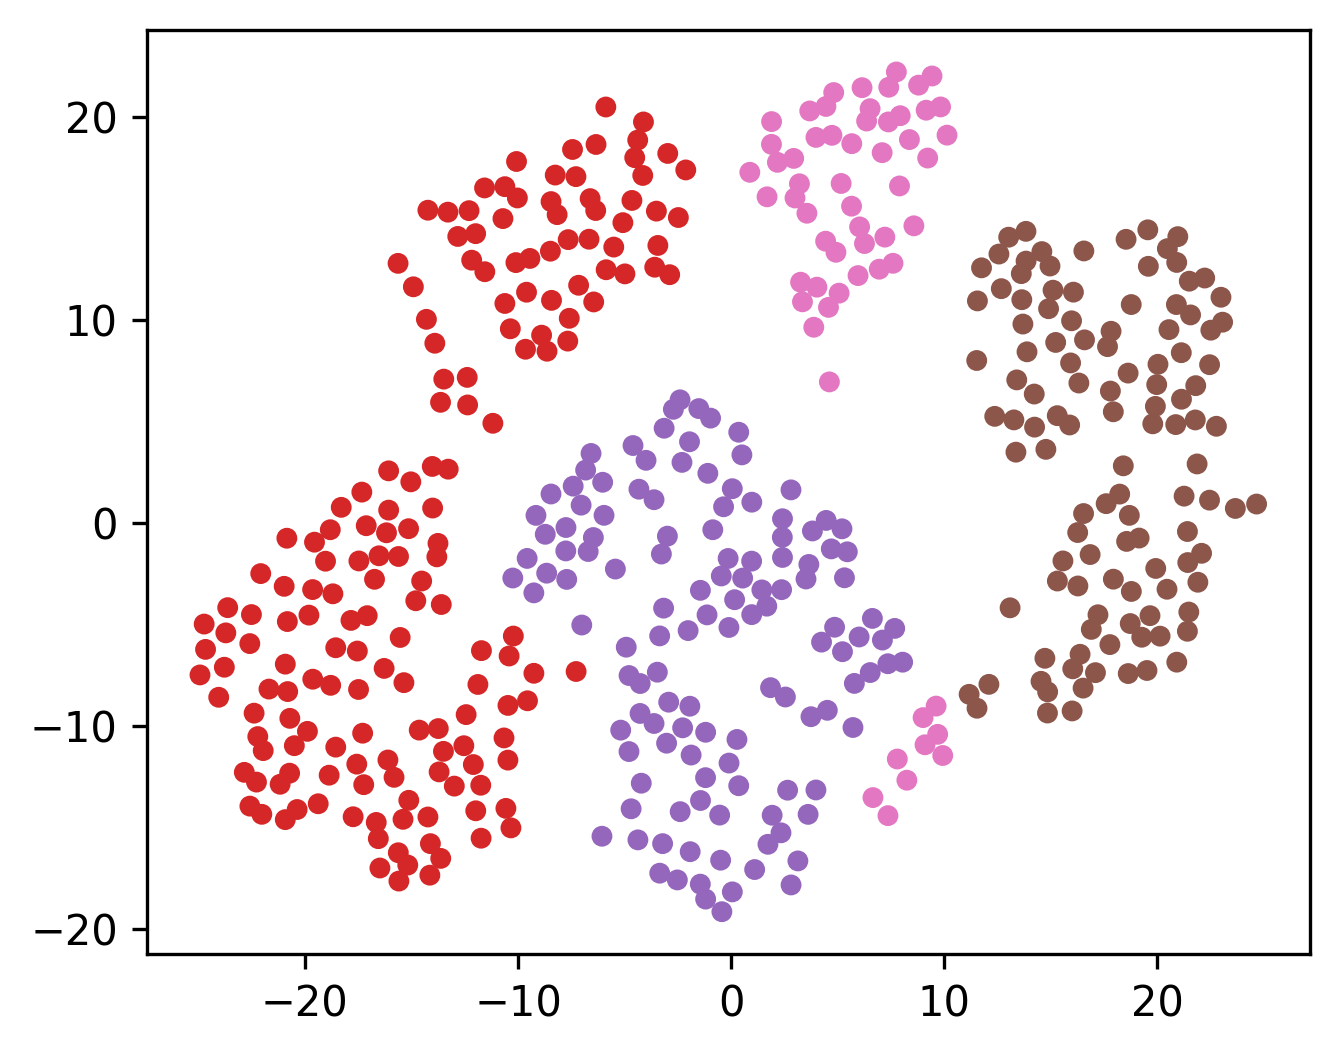}
                \caption{Arrived nodes at the leaf layer.}
                \label{fig:prototypes-2}
        \end{subfigure}
        \begin{subfigure}{0.32\textwidth}
                \includegraphics[width=\textwidth]{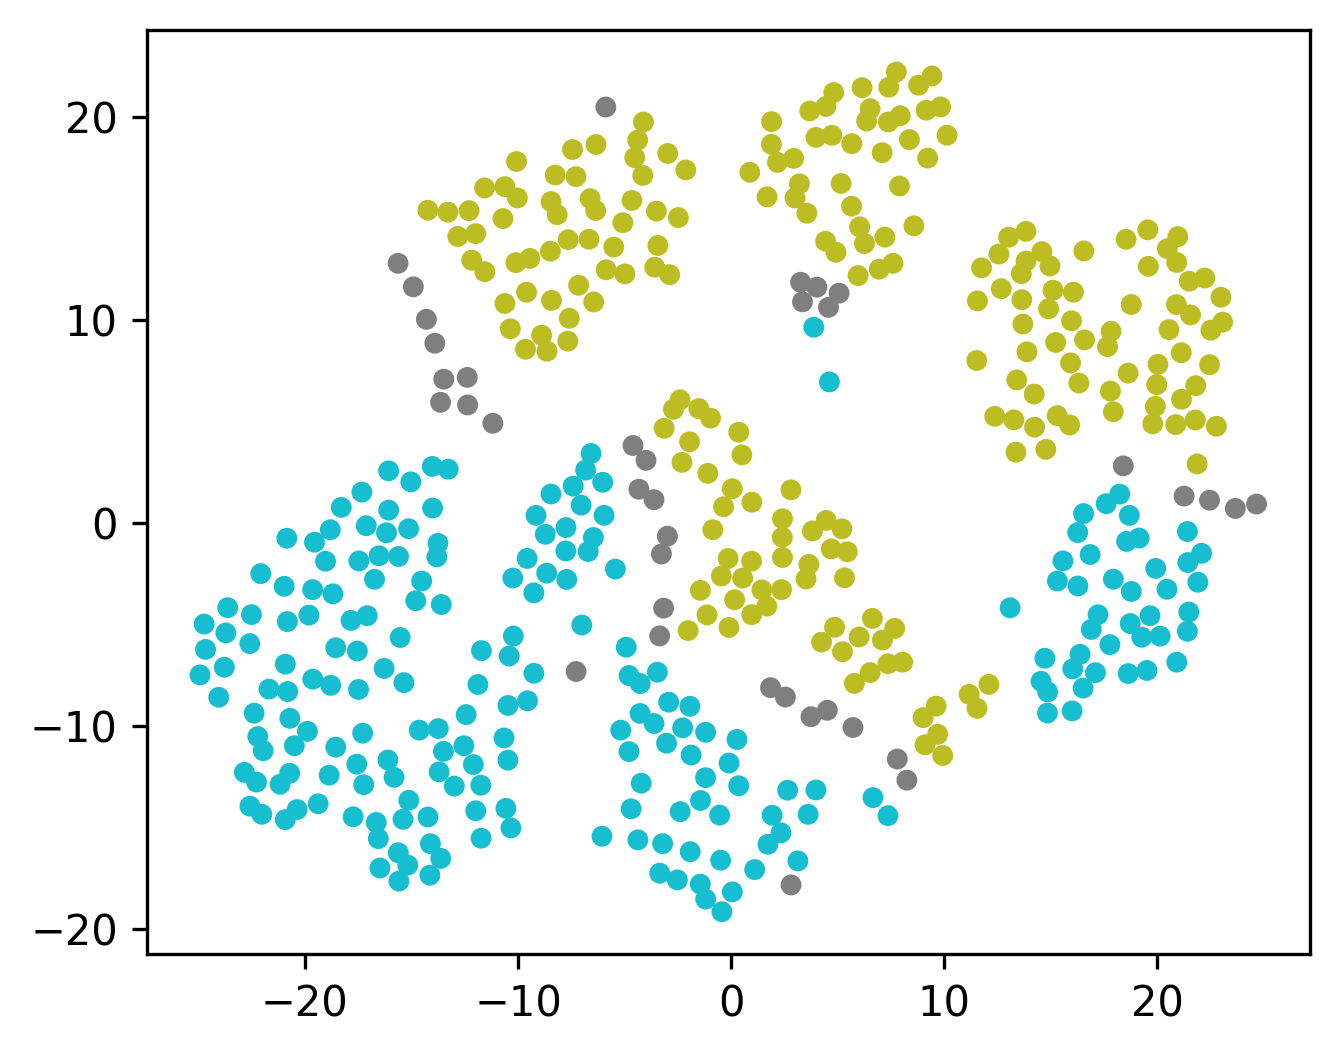}
                \caption{True labels.}
                \label{fig:prototypes-3}
        \end{subfigure}
        
        \caption{%
                t-SNE visualizations of the \texttt{balance-scale} dataset, following the decision process of {\method}-B.
                Each point represents an example, and the color represents the (a) arrived node at layer 1, (b) arrived node at the leaf layer, and (c) true label.
                The examples are split into the leaf nodes as shown in (b) to help drawing decision boundaries at each subset.
%               Note that {\method}-B is a binary tree of depth two, but only three clusters exist in Figure \ref{fig:prototypes-2}.
        }
\label{fig:prototypes}
\end{figure*}

\begin{lemma}
	Assume that $v_1$ and $v_2$ are generated from piecewise linear functions.
	Then, given $r_k(v_1)$ and $r_k(v_2)$, $r_k(v_1 + v_2) = r_k(v_1) + r_k(v_2)$.
\label{prop:addition}
\end{lemma}

\begin{proof}
	We rewrite $r_k(v_1 + v_2)$ as
	\begin{align*}
		r_k(v_1 + v_2) = \frac{\partial (v_1 + v_2)}{\partial x_k} x_k = \frac{\partial v_1}{\partial x_k} x_k + \frac{\partial v_2}{\partial x_k} x_k.
	\end{align*}
	We prove the lemma by applying Equation \eqref{eq:simplified-relevance}.
\end{proof}

\begin{lemma}
	Assume that $v_1$ and $v_2$ are generated from piecewise linear functions.
	Then, given $r_k(v_1)$ and $r_k(v_2)$, $r_k(v_1 v_2) = (v_2 r_k(v_1) + v_1 r_k(v_2)) / 2$.
\label{prop:multiplication}
\end{lemma}

\begin{proof}
	We rewrite $r_k(v_1 v_2)$ as
	\begin{align*}
		r_k(v_1 v_2) = \frac{\partial (v_1 v_2)}{\partial x_k} x_k = \frac{\partial v_1}{\partial x_k} v_2 x_k + \frac{\partial v_2}{\partial x_k} v_1 x_k.
	\end{align*}
	We prove the lemma by applying Equation \eqref{eq:simplified-relevance}, after dividing the outputs by two.
\end{proof}

\begin{theorem}
	\method $\mathcal{M}$ is interpretable if all of its transition functions $\mathcal{T}_1, \cdots, \mathcal{T}_D$ are interpretable, where $D$ is the tree depth.
	\label{theorem:interpretability}
\end{theorem}

\begin{proof}
	In \method, the transition functions are stacked linearly, and the relevance scores are propagated from the root to the leaves through addition and multiplication.
	We perform the mathematical induction:
	\begin{itemize}
		\item \textbf{Base case.}
			The initial probability $\mathbf{p}_0$ is interpretable, since it is a constant.
		\item \textbf{Inductive step.}
			Assume that $\mathbf{p}_d$ is interpretable and the relevance $r_k(p_{d, i})$ is given for all $k$ and $i$.
			Then, $r_k(p_{d+1,j})$ for $\mathbf{p}_{d+1}$ is derived as
			\begin{equation*}
				r_k(p_{d+1,j}) = \frac{1}{2} \sum_i p_{d, i} r_k(t_{d, ji}) + t_{d, ji} r_k(p_{d, i}).
			\end{equation*}
	\end{itemize}
	Thus, the output of $\mathcal{M}$ is also interpretable.
\end{proof}

%\subsection{Interpretability (Q3)}

%We present the interpretability of \method on our datasets by a) the feature relevance scores and b) the visualization of data clusters that are separated into multiple leaf nodes.

\subsection{Feature Relevances}

Tree models provide interpretability via feature relevances as shown in Theorem \ref{theorem:interpretability}.
We assume that every decision function can generate feature relevances by a simple approach to derive the feature relevances of a softmax classifier \cite{Montavon18}.
Consider a function $f(\mathbf{x}) = \mathrm{softmax}(\mathbf{W}\mathbf{x} + \mathbf{b})$.
Then, the relevance of each element $x_k$ is given as
\begin{equation}
        r_k(f_i(\mathbf{x})) = \frac{\max(w_{ki} x_i, 0)}{\sum_j \max(w_{kj} x_k, 0)} f_i(\mathbf{x}).
\label{eq:softmax-relevance}
\end{equation}
This applies also to a binary classifier $f$ that uses a sigmoid activation function.

Afterward, based on the interpretation rule of Equation \eqref{eq:softmax-relevance}, we compare the feature relevances generated from LR and {\method}-A, which are based on generalized linear decisions with either the softmax or a sigmoid function.
Figure \ref{fig:relevances} shows the result on the \texttt{car} dataset for 15 examples randomly selected from the dataset.
Even though {\method}-A makes more complex decisions based on the tree structure, the generated relevances are similar to those of the logistic regression.
This implies that our \method produces consistent predictions whose interpretation matches that of the logistic regression.

Figure \ref{fig:class-relevances} elaborates on the feature relevances by averaging the scores of all examples for each target class.
The patterns are similar to those of Figure \ref{fig:relevances}, but the difference is that this provides more general knowledge about the relations between features and labels, enlarging our understanding of the dataset without given any prior knowledge.
For instance, feature 1 is essential for determining classes 5 and 6, indicated by both of the models, while features 3 and 5 have negligible effects for decisions of all classes.

\subsection{Data Prototypes}

The main advantage of tree models is the generation of subsets of examples, each of which makes a meaningful cluster of data examples.
A notable difference from previous tree models is that each leaf node is modeled as a classifier, rather than a fixed distribution.
Thus, the decision process of our \method is for making easy subsets for each leaf node to easily draw decision boundaries between the given examples, rather than performing classification directly.

Figure \ref{fig:prototypes} visualizes the examples of the \texttt{balance-scale} dataset, following the decision process of {\method}-B.
They are first split in Figure \ref{fig:prototypes-1} by the root node and then distributed to the four leaf nodes as shown in Figure \ref{fig:prototypes-2}.
It is notable that the examples arrived at each leaf node contain all three classes, but their decision boundaries are drawn easily on each subset.
This implies that \method combines the power of tree decisions and leaf classification as a single end-to-end framework.
